# Supplementary material for: Computational Screening of Current Collectors for Enabling Anode-free Lithium Metal Batteries
Source: arXiv:1909.02404 source file (2019-08-21)
Supplement: Supplementary file 1 [file SI_AF.pdf]

# Supporting Information for: Computational Screening of Current Collectors for enabling Anode-free Lithium Metal Batteries

Vikram Pande and Venkatasubramanian Viswanathan*

*Department of Mechanical Engineering, Carnegie Mellon University, Pittsburgh, Pennsylvania 15213, USA*

E-mail: venkvis@cmu.edu

## Anode-free Battery Configuration

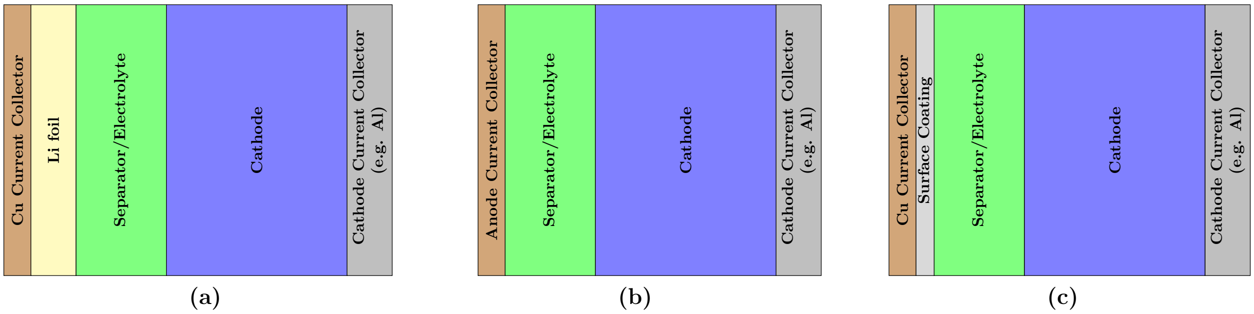


Figure S1: The anode free battery configurations (b) and (c) used compared to the standard Li metal battery configuration shown in (a). (b) employs a new current collector material and (c) employs a new coating material on the standard current collectors such as Cu, Ti, etc. (b) can also result in increase in specific energy of the cell.

## Comparison of Surface Energies to Existing Literature

The Li(100) surface energy determined by BEEF-vdW (0.56 J/m$^2$) is very close to the experimental value of 0.525 J/m$^2$.[1] All Li surface energies are also close to the values reported in prior computational work.[2,3] However we do see change in the order of stability of the facets. We attribute this to the uncertainty associated with the exchange-correlation functional in

Table S1: List of surface energies calculated using BEEF-vdW for the different simulated transition metal surfaces that do not alloy with Li.

| Metal | Surface Miller Indices | Surface Energy ($J/m^2$) |
|---|---|---|
| Cu | (100) | 2.01 |
| Cu | (110) | 1.93 |
| Cu | (111) | 1.40 |
| Cr | (100) | 2.59 |
| Cr | (110) | 2.62 |
| Cr | (111) | 2.63 |
| Fe | (100) | 2.37 |
| Fe | (110) | 2.35 |
| Fe | (111) | 2.06 |
| Mo | (100) | 3.36 |
| Mo | (110) | 2.92 |
| Mo | (111) | 2.80 |
| Ni | (100) | 2.40 |
| Ni | (110) | 2.42 |
| Ni | (111) | 1.70 |
| V | (100) | 2.72 |
| V | (110) | 2.52 |
| V | (111) | 2.30 |
| W | (100) | 4.28 |
| W | (110) | 3.41 |
| W | (111) | 3.42 |
| Zr | (0001) | 1.54 |
| Zr | $(10\bar{1}0)$ | 1.77 |
| Zr | $(10\bar{1}1)$ | 1.64 |
| Zr | $(11\bar{2}0)$ | 1.81 |
| Zr | $(11\bar{2}1)$ | 1.68 |
| Mn | (100) | 3.50 |
| Mn | (110) | 3.62 |
| Mn | (111) | 3.11 |
| Ti | (0001) | 1.85 |
| Ti | $(10\bar{1}0)$ | 2.12 |
| Ti | $(10\bar{1}1)$ | 2.46 |
| Ti | $(11\bar{2}0)$ | 2.01 |
| Ti | $(11\bar{2}1)$ | 1.91 |
| Li | (100) | 0.56 |
| Li | (110) | 0.47 |
| Li | (111) | 0.53 |

DFT. For the fcc metals Cu and Ni, we do predict (111) surface as the most stable surface in agreement to previous literature and the surface energies are about 0.3 J/m$^2$ apart from the experimental values. As expected for hcp crystal Ti and Zr, we predict the (0001) surface to most stable and our values agree very well with experiments which are 2.0 and 2.1 J/m$^2$ for Zr and Ti respectively.[1] For bcc crystals Cr, W, V we get (110) and (111) to be almost equally stable and within 0.3 J J/m$^2$ of the experimental values.[1] Surprisingly for bcc Fe and Mo we get (111) to be more stable than (110) different than prior work.[2,3] However the (110) surface energies are very close to the experimental values.[1] Thus in general our DFT calculations predict sufficiently accurate surface energies for metals and we will use this to analyze the Li-alloy surface energies as well.

## References


(1) Tyson, W.; Miller, W. Surface free energies of solid metals: Estimation from liquid surface tension measurements. *Surf. Sci.* **1977**, *62*, 267–276.

(2) Vitos, L.; Ruban, A.; Skriver, H. L.; Kollar, J. The surface energy of metals. *Surf. Sci.* **1998**, *411*, 186–202.

(3) Skriver, H. L.; Rosengaard, N. Surface energy and work function of elemental metals. *Phys. Rev. B* **1992**, *46*, 7157.

Table S2: List of surface energies calculated using BEEF-vdW for the different simulated Li alloy surfaces.

| Alloy Phase | Surface Miller Indices | Surface Energy ($J/m^2$) |
|---|---|---|
| LiZn | (100) | 0.88 |
| LiZn | (110) | 0.88 |
| LiZn | (111) | 1.07 |
| $Li_3Cd$ | (100) | 0.64 |
| $Li_3Cd$ | (110) | 0.66 |
| $Li_3Cd$ | (111) | 0.69 |
| $Li_3Ag$ | (001) | 0.66 |
| $Li_3Ag$ | (100) | 0.65 |
| $Li_3Ag$ | (101) | 0.77 |
| $Li_3Ag$ | (110) | 0.68 |
| $Li_3Ag$ | (111) | 0.64 |
| $Li_2Ga$ | (001) | 0.82 |
| $Li_2Ga$ | (010) | 1.19 |
| $Li_2Ga$ | (011) | 1.12 |
| $Li_2Ga$ | (100) | 0.84 |
| $Li_2Ga$ | (101) | 0.85 |
| $Li_2Ga$ | (110) | 1.34 |
| $Li_2Ga$ | (111) | 0.84 |
| $Li_9Al_4$ | (001) | 1.26 |
| $Li_9Al_4$ | (010) | 0.90 |
| $Li_9Al_4$ | (011) | 1.02 |
| $Li_9Al_4$ | (100) | 0.82 |
| $Li_9Al_4$ | (101) | 0.89 |
| $Li_9Al_4$ | (110) | 0.96 |
| $Li_9Al_4$ | (111) | 0.97 |
| LiB | (0001) | 1.61 |
| LiB | $(10\bar{1}0)$ | 0.79 |
| LiB | $(10\bar{1}1)$ | 0.94 |
| LiB | $(11\bar{2}0)$ | 0.95 |
| LiB | $(11\bar{2}1)$ | 1.49 |

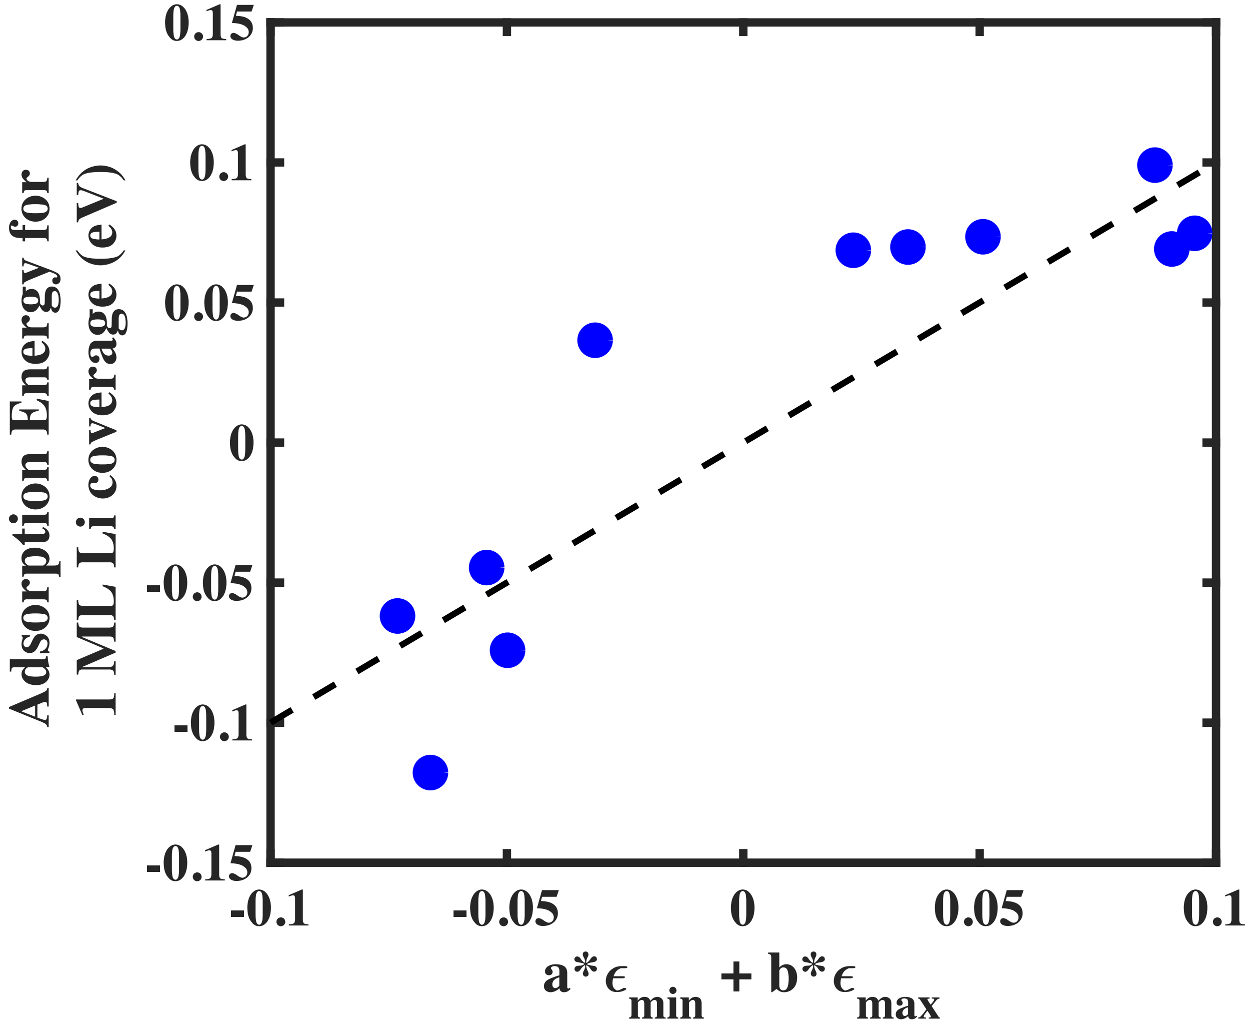


Figure S2: Correlation between the Li adsorption energies at 1M coverage on Li alloys and the strain on the Li atoms on the Li alloy surface calculated with reference to bulk Li. $\epsilon_{min}$ and $\epsilon_{max}$ are the strains in the two unit cell directions on the Li atoms. We find a = -2.75 and b = 1.72 for the best fit.

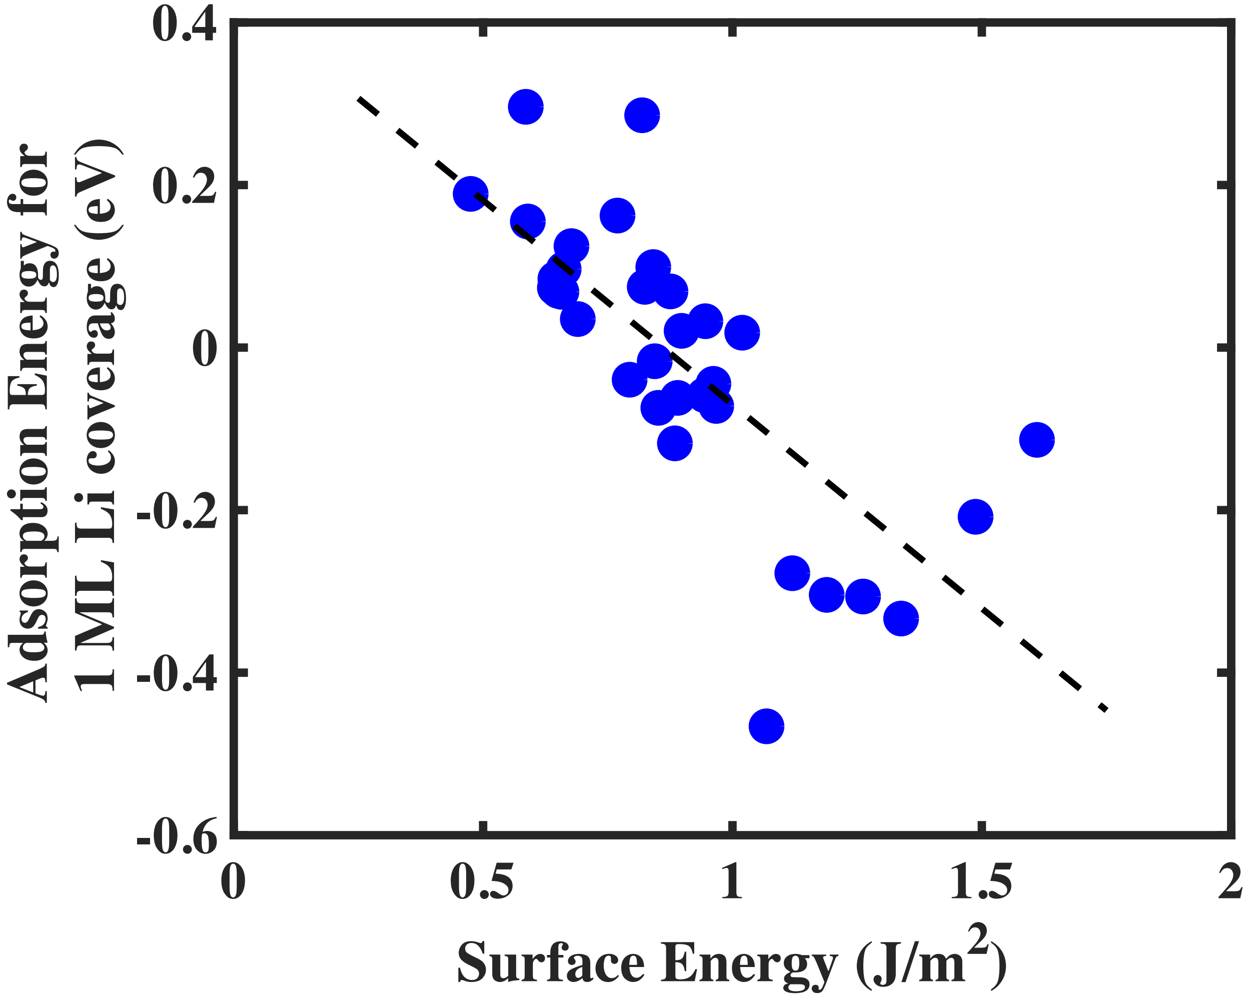


Figure S3: Correlation between the Li adsorption energies at 1M coverage on various Li alloys surfaces with their surface energies.

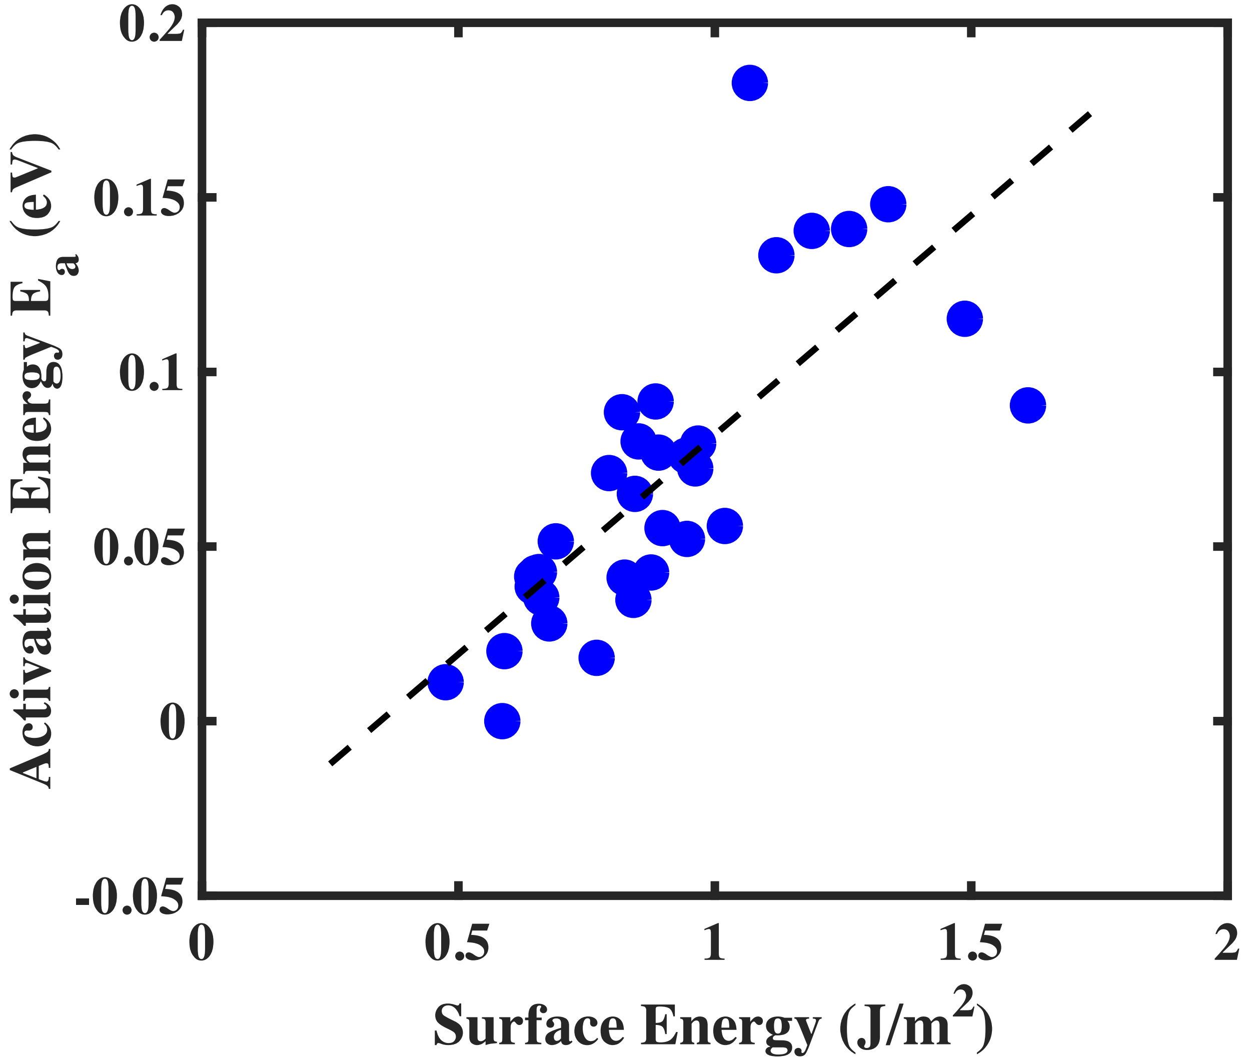


Figure S4: Correlation between the Li surface diffusion activation energies on various Li alloys surfaces with their surface energies.
